# Supplementary material for: Data Dissemination in Cognitive Radio Networks
Source: arXiv:1107.4950 source file (2011-07-25)
Supplement: Supplementary file 1 [file appendix.tex]

\appendix
\lhead[\fancyplain{}{\sl\thepage}]{\fancyplain{}{\sl\rightmark}}
\chead[\fancyplain{}{\sl\leftmark}]{\fancyplain{}{}}
\rhead[\fancyplain{}{\sl Appendix
\thechapter}]{\fancyplain{}{\sl\thepage}}
%\newpage

%========================================================
%% Resumé en français de la thèse
%% ----- Formattage Général

\pagestyle{fancyplain}

\lhead[\fancyplain{}{\sl\thepage}]{\fancyplain{}{\sl\rightmark}}
\chead[\fancyplain{}{\sl\leftmark}]{\fancyplain{}{}}
\rhead[\fancyplain{}{\sl Chapitre
\thechapter}]{\fancyplain{}{\sl\thepage}}

\ifnumcont\else \setcounter{page}{1} \pagenumbering{arabic} \fi

\normalsize

The ZigBee stack architecture ...
